# Supplementary material for: Preference-Learning Emitters for Mixed-Initiative Quality-Diversity Algorithms
Source: arXiv:2210.13839 source file (2023-04-15)
Supplement: Supplementary file 1 [file 10_appendix.tex]

%\newpage

%\appendix

    %\begin{figure*}
    %    \centering
    %    \includegraphics[width=1\textwidth]{images/ui/UI_devmode_preview.jpg}
    %    \caption{Screenshot of the AI Spaceship Generator application in developer mode. In this mode the user has access to most of the underlying components of the generative algorithm.}
    %    \label{fig:webapp-developer}
    %\end{figure*}

    %\begin{figure*}
    %    \centering
    %    \includegraphics[width=1\textwidth]{images/ui/UI_userstudy_preview.jpg}
    %    \caption{Screenshot of the AI Spaceship Generator application in user-study mode mid-generation. In this mode the user is restricted to selecting parent ships for the hybrid EA. Progress bars are used to indicate the current completion status of the user study.}
    %    \label{fig:webapp-user-study}
    %\end{figure*}

    %\begin{figure*}
    %    \centering
    %    \includegraphics[width=1\textwidth]{images/ui/UI_comparator_preview.jpg}
    %    \caption{Screenshot of the Spaceships Ranker application. Users upload their favourite spaceship from the 4 emitter settings within the user study and rank them to provide preference feedback.}
    %    \label{fig:webapp-comparator}
    %\end{figure*}
